# Supplementary material for: Spin precession and spin waves in a chiral electron gas: beyond Larmor's theorem
Source: arXiv:1612.04314 source file (2016-12-13)
Supplement: Supplementary file 1 [file Supplementary.pdf]

# Supplementary information for:
# Spin precession and spin waves in a chiral electron gas: beyond Larmor's theorem

Shahrzad Karimi,[1] Florent Baboux,[2] Florent Perez,[2,3] Carsten A. Ullrich,[1] Grzegorz Karczewski,[4] and Tomasz Wojtowicz[4]

[1]*Department of Physics and Astronomy, University of Missouri-Columbia, Columbia, Missouri, 65211*
[2]*Institut des Nanosciences de Paris, CNRS/Université Paris VI, Paris 75005, France*
[3]*Laboratoire de Photonique et de Nanostructures, LPN/CNRS, 91460 Marcoussis, France*
[4]*Institute of Physics, Polish Academy of Sciences, Warsaw, Poland*
(Dated: December 13, 2016)

In this supplementary section we provide technical details of the derivation of Eq. (6) in the main paper, using the linear-response formalism described in Sec. IV.

The spin-flip response function [Eq. (49) in the main paper] is given by

$$\chi_{\sigma\sigma',\tau\tau'}(\mathbf{q},y,y',\omega) = F_{\sigma\sigma',\tau\tau'}(\mathbf{q},\omega)\phi^2(y)\phi^2(y') ,$$

where

$$\begin{aligned} F_{\sigma\sigma',\tau\tau'}(\mathbf{q},\omega) = &-\sum_{pp'}^{\pm 1}\int\frac{d^2k}{(2\pi)^2}\,\frac{f(E_{p\mathbf{k}})}{\omega - E_{p\mathbf{k}} + E_{p'\mathbf{k-q}} + i\eta} \\ &\left[\delta_{\sigma\uparrow}\psi_{\mathbf{k}}^{p\uparrow} + \delta_{\sigma\downarrow}\psi_{\mathbf{k}}^{p\downarrow}\right]\left[\delta_{\sigma'\uparrow}\psi_{\mathbf{k-q}}^{p'\uparrow} + \delta_{\sigma'\downarrow}\psi_{\mathbf{k-q}}^{p'\downarrow}\right] \\ &\left[\delta_{\tau\uparrow}\psi_{\mathbf{k}}^{p\uparrow} + \delta_{\tau\downarrow}\psi_{\mathbf{k}}^{p\downarrow}\right]\left[\delta_{\tau'\uparrow}\psi_{\mathbf{k-q}}^{p'\uparrow} + \delta_{\tau'\downarrow}\psi_{\mathbf{k-q}}^{p'\downarrow}\right] \\ &+\sum_{pp'}^{\pm 1}\int\frac{d^2k}{(2\pi)^2}\,\frac{f(E_{p\mathbf{k}})}{\omega + E_{p\mathbf{k}} - E_{p'\mathbf{k+q}} + i\eta} \\ &\left[\delta_{\sigma\uparrow}\psi_{\mathbf{k+q}}^{p'\uparrow} + \delta_{\sigma\downarrow}\psi_{\mathbf{k+q}}^{p'\downarrow}\right]\left[\delta_{\sigma'\uparrow}\psi_{\mathbf{k}}^{p\uparrow} + \delta_{\sigma'\downarrow}\psi_{\mathbf{k}}^{p\downarrow}\right] \\ &\left[\delta_{\tau\uparrow}\psi_{\mathbf{k+q}}^{p'\uparrow} + \delta_{\tau\downarrow}\psi_{\mathbf{k+q}}^{p'\downarrow}\right]\left[\delta_{\tau'\uparrow}\psi_{\mathbf{k}}^{p\uparrow} + \delta_{\tau'\downarrow}\psi_{\mathbf{k}}^{p\downarrow}\right] . \end{aligned} \quad (1)$$

The energy eigenvalues to second order in spin-orbit coupling are as follows:

$$E_{p\mathbf{k}} = \frac{k^2}{2} + \frac{\varepsilon_\uparrow + \varepsilon_\downarrow}{2} + \frac{p}{2}\left(Z^* - \mathbf{k}\cdot\mathbf{q}_0 + \frac{(\mathbf{k}\cdot\mathbf{q}_1)^2}{2Z^*}\right).$$

Recall that

$$\mathbf{q}_0 = 2\begin{pmatrix}\alpha\cos\varphi + \beta\sin\varphi \\ \alpha\sin\varphi + \beta\cos\varphi \\ 0\end{pmatrix}$$

$$\mathbf{q}_1 = 2\begin{pmatrix}-\alpha\sin\varphi + \beta\cos\varphi \\ \alpha\cos\varphi - \beta\sin\varphi \\ 0\end{pmatrix}$$

so

$$\begin{aligned} \mathbf{k}\cdot\mathbf{q}_0 &= 2k[\alpha\cos(\varphi - \varphi_k) + \beta\sin(\varphi + \varphi_k)] \\ \mathbf{k}\cdot\mathbf{q}_1 &= -2k[\alpha\sin(\varphi - \varphi_k) - \beta\cos(\varphi + \varphi_k)]. \end{aligned}$$

The single-particle states are real and given to second order in spin-orbit by

$$\psi_+ = \begin{pmatrix} 1 - \frac{(\mathbf{k}\cdot\mathbf{q}_1)^2}{8Z^{*2}} \\ \frac{\mathbf{k}\cdot\mathbf{q}_1}{2Z^*} + \frac{(\mathbf{k}\cdot\mathbf{q}_0)(\mathbf{k}\cdot\mathbf{q}_1)}{2Z^{*2}} \end{pmatrix}\phi(y)$$

$$\psi_- = \begin{pmatrix} -\frac{\mathbf{k}\cdot\mathbf{q}_1}{2Z^*} - \frac{(\mathbf{k}\cdot\mathbf{q}_0)(\mathbf{k}\cdot\mathbf{q}_1)}{2Z^{*2}} \\ 1 - \frac{(\mathbf{k}\cdot\mathbf{q}_1)^2}{8Z^{*2}} \end{pmatrix}\phi(y) .$$

We abbreviate

$$h_{1\mathbf{k}} = \frac{\mathbf{k}\cdot\mathbf{q}_1}{Z^*} .$$

We are interested in the spin-flip waves at $q = 0$. The response function (1) at $q = 0$ can be written in the following way:

$$\begin{aligned} \underline{\underline{F}}(0,\omega) = &-\int\frac{d^2k}{(2\pi)^2}\,\frac{f(E_{+\mathbf{k}})}{\omega - E_{+\mathbf{k}} + E_{-\mathbf{k}} + i\eta}\,\underline{\underline{R}}^+ \\ &+\int\frac{d^2k}{(2\pi)^2}\,\frac{f(E_{+\mathbf{k}})}{\omega + E_{+\mathbf{k}} - E_{-\mathbf{k}} + i\eta}\,\underline{\underline{R}}^- \\ &-\int\frac{d^2k}{(2\pi)^2}\,\frac{f(E_{-\mathbf{k}})}{\omega - E_{-\mathbf{k}} + E_{+\mathbf{k}} + i\eta}\,\underline{\underline{R}}^- \\ &+\int\frac{d^2k}{(2\pi)^2}\,\frac{f(E_{-\mathbf{k}})}{\omega + E_{-\mathbf{k}} - E_{+\mathbf{k}} + i\eta}\,\underline{\underline{R}}^+ \end{aligned}$$

where the matrices $\underline{\underline{R}}^+$ and $\underline{\underline{R}}^-$ are given by

$$\underline{\underline{R}}^+ = \begin{pmatrix} h_{1\mathbf{k}}^2 & -h_{1\mathbf{k}} & 0 & -h_{1\mathbf{k}}^2 \\ -h_{1\mathbf{k}} & 1 - 2h_{1\mathbf{k}}^2 & -h_{1\mathbf{k}}^2 & h_{1\mathbf{k}} \\ 0 & -h_{1\mathbf{k}}^2 & 0 & 0 \\ -h_{1\mathbf{k}}^2 & h_{1\mathbf{k}} & 0 & h_{1\mathbf{k}}^2 \end{pmatrix}$$

$$\underline{\underline{R}}^- = \begin{pmatrix} h_{1\mathbf{k}}^2 & 0 & -h_{1\mathbf{k}} & -h_{1\mathbf{k}}^2 \\ 0 & 0 & -h_{1\mathbf{k}}^2 & 0 \\ -h_{1\mathbf{k}} & -h_{1\mathbf{k}}^2 & 1 - 2h_{1\mathbf{k}}^2 & h_{1\mathbf{k}} \\ -h_{1\mathbf{k}}^2 & 0 & h_{1\mathbf{k}} & h_{1\mathbf{k}}^2 \end{pmatrix}.$$

Now let us calculate the energy in the denominator and drop the $i\eta$. We have

$$\begin{aligned} &\underline{\underline{F}}(0,\omega) \\ &= \int\frac{d^2k}{(2\pi)^2}\left[\frac{f(E_{-\mathbf{k}})}{\omega - Z^* + g_0 - g_1} - \frac{f(E_{+\mathbf{k}})}{\omega - Z^* + g_0 - g_1}\right]\underline{\underline{R}}^+ \\ &+ \int\frac{d^2k}{(2\pi)^2}\left[\frac{f(E_{+\mathbf{k}})}{\omega + Z^* - g_0 + g_1} - \frac{f(E_{-\mathbf{k}})}{\omega + Z^* - g_0 + g_1}\right]\underline{\underline{R}}^- \end{aligned}$$

$$= \frac{1}{\omega - Z^*} \int \frac{d^2k}{(2\pi)^2} \frac{f(E_{-\mathbf{k}}) - f(E_{+\mathbf{k}})}{1 + \frac{g_0 - g_1}{\omega - Z^*}} \underline{\underline{R}}^+$$
$$\frac{1}{\omega + Z^*} \int \frac{d^2k}{(2\pi)^2} \frac{f(E_{+\mathbf{k}}) - f(E_{-\mathbf{k}})}{1 + \frac{-g_0 + g_1}{\omega + Z^*}} \underline{\underline{R}}^- ,$$

where

$$g_0 = 2\mathbf{k}\cdot\mathbf{q}_0 , \qquad g_1 = \frac{2(\mathbf{k}\cdot\mathbf{q}_1)^2}{Z^*} .$$

Next, we expand the integrands of $F^{sf}_{\sigma\sigma',\tau\tau'}(0,\omega)$ up to second order in spin-orbit coupling, and carry out the integration over $\mathbf{k}$ for each element of the $4\times 4$ matrices $\underline{\underline{R}}^+$ and $\underline{\underline{R}}^-$. We use a notation where $F_0^\pm$, $F_1^\pm$, and $F_2^\pm$ come from those terms containing zeroth, first and second order in $h_{1\mathbf{k}}$, respectively. After a lengthy calculation, the result is

$$\underline{\underline{F}}(0,\omega) = \begin{pmatrix} F_2^+ + F_2^- & -F_1^+ & -F_1^- & -F_2^+ - F_2^- \\ -F_1^+ & F_0^+ - 2F_2^+ & -F_2^+ - F_2^- & F_1^+ \\ -F_1^- & -F_2^+ - F_2^- & F_0^- - 2F_2^- & F_1^- \\ -F_2^+ - F_2^- & F_1^+ & F_1^- & F_2^+ + F_2^- \end{pmatrix}$$

where

$$F_0^\pm = \frac{\pm Z^*}{2\pi(\omega \mp Z^*)} \pm \frac{N_s(a-b)}{Z^*(\omega \mp Z^*)} + \frac{2N_s(a+b)}{(\omega \mp Z^*)^2} + \frac{N_s(a-b)}{(\omega \mp Z^*)^2} \pm \frac{2N_s Z^*(a+b)}{(\omega \mp Z^*)^3}$$
$$F_1^\pm = \mp c N_s \left[ \frac{1}{Z^*(\omega \mp Z^*)} \pm \frac{1}{(\omega \mp Z^*)^2} \right]$$
$$F_2^\pm = \frac{\pm N_s(a-b)}{2Z^*(\omega \mp Z^*)}$$

and $a = \alpha^2 + \beta^2$, $b = 2\alpha\beta \sin 2\varphi$ and $c = 2\alpha\beta\cos(2\varphi)$.

Instead of the spin-density-matrix response, we will work with density-magnetization response [Eq. (52) in the main paper]. Further details can be found in the Appendix of Ref. 1. It follows that all contributions to the density channel vanish, and the remaining nonvanishing terms of the density-magnetization response function are

$$\begin{aligned}
\Pi_{11} &= \chi_{\uparrow\downarrow\uparrow\downarrow} + \chi_{\uparrow\downarrow\downarrow\uparrow} + \chi_{\downarrow\uparrow\uparrow\downarrow} + \chi_{\downarrow\uparrow\downarrow\uparrow} \\
\Pi_{12} &= -i(\chi_{\uparrow\downarrow\uparrow\downarrow} - \chi_{\uparrow\downarrow\downarrow\uparrow} + \chi_{\downarrow\uparrow\uparrow\downarrow} - \chi_{\downarrow\uparrow\downarrow\uparrow}) \\
\Pi_{13} &= \chi_{\uparrow\downarrow\uparrow\uparrow} - \chi_{\uparrow\downarrow\downarrow\downarrow} + \chi_{\downarrow\uparrow\uparrow\uparrow} - \chi_{\downarrow\uparrow\downarrow\downarrow} \\
\Pi_{21} &= i(\chi_{\uparrow\downarrow\uparrow\downarrow} + \chi_{\uparrow\downarrow\downarrow\uparrow} - \chi_{\downarrow\uparrow\uparrow\downarrow} - \chi_{\downarrow\uparrow\downarrow\uparrow}) \\
\Pi_{22} &= \chi_{\uparrow\downarrow\uparrow\downarrow} - \chi_{\uparrow\downarrow\downarrow\uparrow} - \chi_{\downarrow\uparrow\uparrow\downarrow} + \chi_{\downarrow\uparrow\downarrow\uparrow} \\
\Pi_{23} &= i(\chi_{\uparrow\downarrow\uparrow\uparrow} - \chi_{\uparrow\downarrow\downarrow\downarrow} - \chi_{\downarrow\uparrow\uparrow\uparrow} + \chi_{\downarrow\uparrow\downarrow\downarrow}) \\
\Pi_{31} &= \chi_{\uparrow\uparrow\uparrow\downarrow} + \chi_{\uparrow\uparrow\downarrow\uparrow} - \chi_{\downarrow\downarrow\uparrow\downarrow} - \chi_{\downarrow\downarrow\downarrow\uparrow} \\
\Pi_{32} &= -i(\chi_{\uparrow\uparrow\uparrow\downarrow} - \chi_{\uparrow\uparrow\downarrow\uparrow} - \chi_{\downarrow\downarrow\uparrow\downarrow} + \chi_{\downarrow\downarrow\downarrow\uparrow}) \\
\Pi_{33} &= \chi_{\uparrow\uparrow\uparrow\uparrow} - \chi_{\uparrow\uparrow\downarrow\downarrow} - \chi_{\downarrow\downarrow\uparrow\uparrow} + \chi_{\downarrow\downarrow\downarrow\downarrow}
\end{aligned}$$

and $\Pi_{00} = \Pi_{01} = \Pi_{02} = \Pi_{03} = \Pi_{10} = \Pi_{20} = \Pi_{30} = 0$. Therefore, the total response function is a $4\times 4$ matrix whose elements defined as follows:

$$\begin{aligned}
\Pi_{11} &= F_0^+ + F_0^- - 4(F_2^- + F_2^+) \\
\Pi_{12} &= -i(F_0^+ - F_0^- - 2F_2^+ + 2F_2^-) \\
\Pi_{13} &= -2(F_1^+ + F_1^-) \\
\Pi_{21} &= i(F_0^+ - F_0^- - 2F_2^+ + 2F_2^-) \\
\Pi_{22} &= F_0^+ + F_0^- \\
\Pi_{23} &= 2i(F_1^- - F_1^+) \\
\Pi_{31} &= -2(F_1^+ + F_1^-) \\
\Pi_{32} &= -2i(F_1^- - F_1^+) \\
\Pi_{33} &= 4(F_2^+ + F_2^-)
\end{aligned}$$

where each element is multiplied with $\phi^2(y)\phi^2(y')$. In order to find the collective modes, we need to determine those frequencies where the matrix

$$\underline{\underline{M}}(\mathbf{q},\omega) = \underline{\underline{H}}^{\rm xc}(\mathbf{q},\omega)\underline{\underline{\Pi}}(\mathbf{q},\omega) \qquad (2)$$

has the eigenvalue 1, where the xc matrix $\underline{\underline{H}}^{\rm xc}$ is given by Eq. (54) in the main paper. In other words, we solve the $4\times 4$ eigenvalue problem

$$\underline{\underline{M}}(\mathbf{q},\omega)\vec{x} = \lambda(\mathbf{q},\omega)\vec{x} \qquad (3)$$

and find the mode frequencies by solving $\lambda(\mathbf{q},\omega) = 1$ for $\omega$, where $\mathbf{q}$ is fixed. Since here our goal is to obtain the coefficient $E_0$ to second order in the Rashba and Dresselhaus coupling strengths $\alpha$ and $\beta$, we carry out a perturbative expansion of the eigenvalue problem (3) in orders of spin-orbit coupling. At $q = 0$, the matrix can be written as

$$\underline{\underline{M}}(0,\omega) = \underline{\underline{M}}^{(0)} + \underline{\underline{M}}^{(2)} + \ldots \qquad (4)$$

where superscripts indicate the order of spin-orbit coupling (the linear order vanishes at $q = 0$).

We now write $\underline{\underline{\Pi}} = \underline{\underline{\Pi}}^{(0)} + \underline{\underline{\Pi}}^{(2)}$, where $\underline{\underline{\Pi}}^{(0)}$ and $\underline{\underline{\Pi}}^{(2)}$ are in zero and second order in spin-orbit coupling, respectively. Let us first work out the zero-order case and solve the zero-order eigenvalue problem $\underline{\underline{M}}^{(0)}\vec{x}^{(0)} = \lambda^{(0)}\vec{x}^{(0)}$. The zero-order response function matrix is

$$\underline{\underline{\Pi}}^{(0)} = \frac{Z^*\phi^2(y)\phi^2(y')}{\pi(\omega^2 - Z^{*2})} \begin{pmatrix} 0 & 0 & 0 & 0 \\ 0 & Z^* & -i\omega & 0 \\ 0 & i\omega & Z^* & 0 \\ 0 & 0 & 0 & 0 \end{pmatrix} . \qquad (5)$$

Now we need to do the multiplication with the xc kernel matrix (see Eq. (3)):

$$\underline{\underline{M}}^{(0)} = \frac{Z^*/\pi}{\omega^2 - Z^{*2}} \begin{pmatrix} h^{\rm xc}_{00} & 0 & 0 & h^{\rm xc}_{03} \\ 0 & h^{\rm xc}_{11} & 0 & 0 \\ 0 & 0 & h^{\rm xc}_{22} & 0 \\ h^{\rm xc}_{30} & 0 & 0 & h^{\rm xc}_{33} \end{pmatrix} \begin{pmatrix} 0 & 0 & 0 & 0 \\ 0 & Z^* & -i\omega & 0 \\ 0 & i\omega & Z^* & 0 \\ 0 & 0 & 0 & 0 \end{pmatrix}$$

The elements of the xc matrix, $h^{ij}_{\rm xc}$, are given in Eqs. (55)-(59) in the main paper, averaged over $\phi^4(y)$. In particular, we find $h^{\rm xc}_{11} = h^{\rm xc}_{22} = \pi f_T$ [see Eq. (63) in the main paper]. When we work this out, we find

$$\underline{\underline{M}}^{(0)} = \frac{Z^* f_T}{\omega^2 - {Z^*}^2} \begin{pmatrix} 0 & 0 & 0 & 0 \\ 0 & Z^* & -i\omega & 0 \\ 0 & i\omega & Z^* & 0 \\ 0 & 0 & 0 & 0 \end{pmatrix}. \tag{6}$$

The spin-flip wave at $q = 0$ is at that frequency where the $4 \times 4$ matrix $\underline{\underline{M}}^{(0)}$ has eigenvalue 1. Working out the determinant leads to the following result:

$$\omega_0 = Z^* + Z^* f_T = Z \tag{7}$$

(there is also a solution with a negative frequency, which we discard). We substitute $\omega_0$ back into Eq. (6), and end up with

$$\underline{\underline{M}}^{(0)} = \begin{pmatrix} 0 & 0 & 0 & 0 \\ 0 & \frac{1}{2+f_T} & -i\frac{1+f_T}{2+f_T} & 0 \\ 0 & i\frac{1+f_T}{2+f_T} & \frac{1}{2+f_T} & 0 \\ 0 & 0 & 0 & 0 \end{pmatrix}.$$

The normalized eigenvector which makes the eigenvalue of $\underline{\underline{M}}^{(0)}$ equal to 1 is

$$\vec{x}^{(0)} = \frac{1}{\sqrt{2}} \begin{pmatrix} 0 \\ -i \\ 1 \\ 0 \end{pmatrix}.$$

To obtain the change of the eigenmodes caused by the presence of spin-orbit coupling, we need to determine $\lambda^{(2)}$. In perturbation theory, we obtain the second-order correction of the eigenvalues as

$$\lambda^{(2)} = [\vec{x}^{(0)}]^\dagger \underline{\underline{M}}^{(2)} \vec{x}^{(0)}, \tag{8}$$

where we can construct $\underline{\underline{M}}^{(2)}$ by using $\underline{\underline{\Pi}}^{(2)}$.

$$\underline{\underline{M}}^{(2)} = \begin{pmatrix} 0 & 0 & 0 & 0 \\ 0 & h^{\rm xc}_{11}\Pi^{(2)}_{11} & h^{\rm xc}_{11}\Pi^{(2)}_{12} & h^{\rm xc}_{11}\Pi^{(2)}_{13} \\ 0 & h^{\rm xc}_{22}\Pi^{(2)}_{21} & h^{\rm xc}_{22}\Pi^{(2)}_{22} & h^{\rm xc}_{22}\Pi^{(2)}_{23} \\ 0 & h^{\rm xc}_{33}\Pi^{(2)}_{31} & h^{\rm xc}_{33}\Pi^{(2)}_{32} & h^{\rm xc}_{33}\Pi^{(2)}_{33} \end{pmatrix}.$$

With the substitution of the terms in second-order in $\alpha$ and $\beta$ in the spin-flip response matrix, $\lambda^{(2)}$ in Eq. (8) will be

$$\begin{aligned} \lambda^{(2)} &= \frac{\pi f_T}{2}(\Pi^{(2)}_{11} + \Pi^{(2)}_{22} + i\Pi^{(2)}_{12} - i\Pi^{(2)}_{21}) \\ &= \pi f_T (2F^+_0 - 4F^+_2) \\ &= \frac{4\pi N_s f_T (a+b)}{(\omega - Z^*)^2} + \frac{2\pi N_s f_T (a-b)}{(\omega - Z^*)^2} \\ &\quad + \frac{4\pi N_s f_T Z^*(a+b)}{(\omega - Z^*)^3}. \end{aligned}$$

To remain within second order of spin-orbit coupling, we substitute $\omega_0$ in Eq. (7) back into $\lambda^{(2)}$, and get

$$\begin{aligned} \lambda^{(2)} &= \frac{6\pi N_s a}{{Z^*}^2 f_T} + \frac{2\pi N_s b}{{Z^*}^2 f_T} + \frac{4\pi N_s Z^*(a+b)}{{Z^*}^3 f_T^2} \\ &= \frac{2\pi N_s}{{Z^*}^2 f_T^2}\left[(\alpha^2+\beta^2)(3f_T+2) + 2\alpha\beta\sin(2\varphi)(f_T+2)\right] \end{aligned} \tag{9}$$

The condition for the spin wave at $q = 0$ is that the eigenvalue is equal to 1, so to second order perturbation theory we have

$$1 = \lambda^{(0)} + \lambda^{(2)},$$

where $\lambda^{(0)}$ is known, so

$$1 = \frac{Z^* f_T}{\omega - Z^*} + \lambda^{(2)}$$

which gives

$$\omega - Z^* = Z^* f_T + \lambda^{(2)}(\omega - Z^*).$$

To lowest order in spin-orbit, we replace $\omega$ on the right-hand side by $\omega_0$:

$$\omega = Z^* + Z^* f_T + \lambda^{(2)}(\omega_0 - Z^*)$$

and using $\omega_0 = Z^* + Z^* f_T$ we obtain

$$\omega = \omega_0 + \lambda^{(2)} Z^* f_T$$

Using expression (9), we obtain the final result

$$\begin{aligned} E_0 = Z + \frac{2\pi N_s}{Z^* f_T}\big[&(\alpha^2+\beta^2)(3f_T+2) \\ &+ 2\alpha\beta\sin(2\varphi)(f_T+2)\big], \end{aligned}$$

which is given as Eq. (6) in the main paper.

[1] C. A. Ullrich and M. E. Flatté, Phys. Rev. B **66**, 205305 (2002)
